# Supplementary material for: Leave No Patient Behind: Enhancing Medication Recommendation for Rare Disease Patients
Source: arXiv:2403.17745 source file (2024-08-11)
Supplement: Supplementary file 1 [file appendix.tex]

\appendix

\section{Additional Experiment Details}

% \subsection{Dataset Processing} \label{apd:data process}
% We used EHR data from MIMIC-III~\cite{mimic-iii}, MIMIC-IV~\cite{mimic-iv} and DDI data extracted from the TWOSIDES database~\cite{ddi}. Following previous works~\cite{gamenet, safedrug}, we processed the datasets and randomly divided them into training, validation, and testing sets in a ratio of 4:1:1.
% During pre-processing We then extracted the top 40 severity DDI types from the TWOSIDES database~\cite{ddi}, and converted the drug coding from the National Drug Code (NDC) to the Anatomical Therapeutic Chemical (ATC) classification system at the third level to ensure compatibility with DDI data. 
% In line with previous research~\cite{gamenet}, we selected a cohort of patients who had more than one visit to enhance the efficiency of the experiment. 

\subsection{Baseline Details} \label{apd:baseline}

We compare RAREMed against the following baseline algorithms:

\begin{itemize}[leftmargin=*]
    \item \textbf{LR} is a standard logistic regression technique, 
    where inputs are represented as a multi-hot vector of length $|\mathcal{D}|+|\mathcal{P}|$.
    % and the recommendation problem is formulated as a multi-label classification task.
    
    \item \textbf{LEAP} \cite{leap} is an instance-based method, which employs the LSTM model to generate medication sequence.
    
    \item \textbf{RETAIN} \cite{retain} is a longitudinal model that utilizes two-level neural attention mechanism to predict patients' future condition.
    % detect influential past visits and significant clinical variables. 
    
    \item \textbf{G-Bert} \cite{g-bert} integrates the GNN representation into transformer-based visit encoders, which is pre-trained on single-visit data.
    
    \item \textbf{GAMENet} \cite{gamenet} uses memory neural networks and graph convolutional networks to encode historical EHR data and DDI graph.
    
    \item \textbf{SafeDrug} \cite{safedrug} leverages the drug molecular graph and DDI graph to ensure the safety of medication recommendations.
    
    \item \textbf{COGNet} \cite{cognet} uses a novel copy-or-predict mechanism which frames drug recommendation as a sequence generation problem.
    % within an encoder-decoder framework.

    \item \textbf{MICRON} \cite{micron} is an recurrent residual learning model that focuses on the change of medications.

    \item \textbf{MoleRec}~\cite{molerec} models 
    % the interaction among molecular substructures and 
    the dependencies between patient's health condition and molecular substructures.
    
    % \item \textbf{COGNet} \cite{cognet} introduces a novel copy-or-predict mechanism for generating medication recommendations. This method decides whether to copy a medicine from previous recommendations or to predict a new one.
    % \item \textbf{MICRON} \cite{micron} is an recurrent residual learning model that considers medication changes as input and then conducts medication recommendation based on the medication changes and the medication combination of the last visit.
\end{itemize}

\subsection{Metrics}\label{apd:metric}

% In this section, we present definitions for each metric employed within the experiment: Jaccard Similarity Score (Jaccard), Precision Recall AUC (PRAUC), F1 score (F1), and DDI rate (DDI). Building upon the formulation detailed in Section~\ref{sec:formulation}, $\mathcal{M}$ represents the set of all medications, while $\mathbf{m}^{(j)}\in \{0, 1\}^{|\mathcal{M}|}$ signifies the medications prescribed to a patient identified by index $j$. For simplicity, we will subsequently omit the superscript $j$ for a single-visit patient, ensuring clarity and avoiding ambiguity.

In this subsection, we define the metrics employed within the experiment: Jaccard Similarity Score (Jaccard), Precision Recall AUC (PRAUC), F1 score (F1), and DDI rate (DDI). Building upon the formulation detailed in Section~\ref{sec:formulation}, $\mathcal{M}$ represents the set of all medications in the dataset, while $\mathbf{m}^{(j)}, \hat{\mathbf{m}}^{(j)}\in \{0, 1\}^{|\mathcal{M}|}$ signify the prescribed and predicted medications to a patient identified by index $j$, respectively. For simplicity, we will subsequently omit the superscript $j$ for a single-visit patient.

\begin{itemize}[leftmargin=*]
    \item \textbf{Jaccard}:
    \begin{align*}
        \text{Jaccard} = \frac{\{i:\mathbf{m}_i=1\}\cap\{j:\hat{\mathbf{m}}_j=1\}}{\{i:\mathbf{m}_i=1\}\cup\{j:\hat{\mathbf{m}}_j=1\}}.
    \end{align*}
    
    \item \textbf{F1}:
    \begin{align*}
        \text{F}_1=\frac{2\text{R}\times \text{P}}{\text{R}+\text{P}},
    \end{align*}
    \noindent where the recall and precision are formulated as
    \begin{align*}
        \text{R}=\frac{\{i:\mathbf{m}_i=1\}\cap\{j:\hat{\mathbf{m}}_j=1\}}{\{i:\mathbf{m}_i=1\}},
        \text{P}=\frac{\{i:\mathbf{m}_i=1\}\cap\{j:\hat{\mathbf{m}}_j=1\}}{\{j:\hat{\mathbf{m}}_j=1\}}.
    \end{align*}
    
    \item \textbf{PRAUC}:
    \begin{align*}
        \text{PRAUC}=\sum_{k=1}^{|\mathcal{M}|}\text{P}_k(\text{R}_k-\text{R}_{k-1}),
    \end{align*}
    \noindent where $\text{P}_k, \text{R}_k$ represent the precision and recall at cut-off $k$.
    
    \item \textbf{DDI}:
    \begin{align*}
        \text{DDI}=\frac{\sum_{l,k\in\{i:\hat{\mathbf{m}}_i=1\}}\mathbf{A}_{lk}}{\sum_{l,k\in\{i:\hat{\mathbf{m}}_i=1\}}1},
    \end{align*}
    where $\mathbf{A}$ is the DDI graph defined in Section~\ref{sec:formulation}.
\end{itemize}
% \subsection{Implementation Details}

% Our RAREMed is pre-trained on training set in a sequential manner, first on the SMP task and then on the SP task. 
% For all baseline methods, we adhere to the parameter settings specified in their respective papers. Hyperparameter selection is performed on the validation set. The transformer encoder consists of 3 layers with 4 attention heads. The pre-training process is conducted for 20 epochs for each task, with an embedding dimension of 512. The weights of the loss function, denoted as $\alpha$ and $\beta$, are set to 0.03 and 0.1, respectively. 
% The parameters are trained using the AdamW optimizer~\cite{adamw} with a learning rate of 1e-5 and weight decay of 0.1. 
% All experiments are conducted on a server with 2 Intel Xeon Gold 5118 CPUs, 8 NVIDIA GeForce RTX 3090 GPUs and 754G RAM.

\begin{table*}[h]\small
    \centering
    \caption{Medication recommendation results for a rare disease patient. Here, "FN" (False Negative) denotes medications present in the ground truth but not predicted, whereas "FP" (False Positive) refers to predicted medications not found in the ground truth. The underlined diseases appear less than 30 times in the experimental dataset.}
    \label{tab:case study}

\begin{tabular}{l|c|l}
\hline
Diagnoses \& Procedures (ICD codes~\cite{icd9}) & Methods & Medication Recommendation (ATC codes~\cite{atc3}) \\ \hline
 & \multirow{2}{*}{Ground Truth} & A02A, N02B, B05C, A12A, A12C, A06A, B01A, A04A, N06A, N05C, B03B, N05A, A02B \\
\textbf{Diagnoses}: \underline{5799, 71943, 5959, 920, 61610,} &  & J01D, N05B, J01E, N06D, A11D, H04A, A12B, N03A, A01A (totally 22 medications) \\ \cline{2-3} 
\underline{30392, 80122, 37941, 8020, 8054, 2811}, 311, & GAMENet & 14 correct, 8 FN (A02A, A11D, A12A, B03B, H04A, J01E, N05C, N06D), 2 FP (A07A, N02A) \\ \cline{2-3} 
E8844, 29420, V1271, 04149, E8809, E8796, & SafeDrug & 16 correct, 6 FN (A02A, A01A, A11D, J01E, N05C, N06D), 3 FP (C07A, N02A, N07B) \\ \cline{2-3} 
27650, V1588, 99664, 29181, 34982, 78791, & MICRON & 17 correct, 5 FN (A02A, J01E, N03A, N05C, N06D), 3 FP (A07A, C07A, N02A) \\ \cline{2-3} 
42789, 2875, 2762, 2809, 2753, 2930 (totally & COGNet & 17 correct,  5 FN (A02A, A12A, J01E, N05C, N06D), 5 FP (A07A, C07A, C10A, R01A, R03A) \\ \cline{2-3} 
30 diseases) & MoleRec & 17 correct, 5 FN (A02A, J01E, N05C, N06A, N06D), 4 FP (A07A, C07A, N02A, N07B)
\\ \cline{2-3} 
 \textbf{Procedures}: 8659, 3897& $w/o$ P & 17 correct,  5 FN (A02A, A11D, J01E, N05C, N06D), 5 FP (A07A, C07A, N02A, N07B, R03A) \\ \cline{2-3} 
 & RAREMed & 19 correct, 3 FN (J01E, N05C, N06D), 2 FP (A07A, N02A) \\ \hline
\end{tabular}

\end{table*}

\section{Exploratory Analysis}

\subsection{Case Study}
\label{sec: case}

% We selected a patient in MIMIC-III from the rare group of the test dataset with the intention of demonstrating RAREMed's effectiveness in handling rare cases. The patient's characteristics are detailed in Table \ref{tab:case study}, where we observed 30 diagnosed diseases, 2 procedures and 22 prescribed medications, in which 11 diseases appear less than 30 times within the dataset.
% In evaluating the RAREMed's performance, we compared the medications prescribed by clinicians with the medications predicted by various baseline models with an ablation variant "$w/o$ P", in which pre-training is removed. Notably, RAREMed outperformed other baselines and "$w/o$ P", achieving 19 accurate predictions. It encountered a mere 3 medication oversights and made 2 incorrect predictions, thereby showcasing its accurate performance in this challenging scenario. The results affirm that our framework provides more comprehensive patient representations, resulting in fewer omissions in recommendations and reduced errors compared to other methods, particularly for patients with less frequently documented medical information.

To demonstrate RAREMed's effectiveness in handling rare cases, we select a patient from the rare group in the test set of MIMIC-III, whose characteristics are detailed in Table \ref{tab:case study}, revealing the presence of 30 diagnosed diseases, 2 procedures, and 22 prescribed medications. Notably, among the diagnosed diseases, 11 of them appear less than 30 times within the dataset, indicating their rarity. We exclude G-Bert~\cite{g-bert} and RETAIN~\cite{retain} as they cannot deal with such single-visit patient.

% We compare the medications prescribed by clinicians with the predictions made by various baseline models, including an ablation variant "$w/o$ P" where pre-training is removed. 
Remarkably, RAREMed outperforms all baselines and the "$w/o$ P" variant, achieving 19 accurate predictions. It encounters only 3 medication oversights and makes 2 incorrect predictions, thereby showcasing its accurate performance in this challenging scenario. 
% These results affirm that RAREMed provides more comprehensive patient representations, resulting in fewer omissions and reduced errors in medication recommendations compared to other methods, particularly for patients with less frequently documented medical information.

Specifically, it is noteworthy that all models, except RAREMed, fail to identify the medication \textbf{A02A}, which corresponds to antacids used to alleviate stomach pain and digestive issues, and holds strong relevance with the disease "unspecified digestive system disorder" (indicated by the ICD code \textbf{5799}). 
% RAREMed stands alone in successfully recommending this medication for patients with such conditions. 
% This observation underscores the robust effectiveness of our model's medication recommendation capabilities, particularly in scenarios involving patients with infrequently occurring health conditions.

% These medications are closely associated with specific digestive disorders such as indigestion and acid reflux. Importantly, within the underlined rare diseases, A02A holds strong relevance with the disease "unspecified digestive system disorder" (indicated by the ICD code 5799). RAREMed stands alone in successfully recommending this medication for patients with such conditions. This observation underscores the robust effectiveness of our model's medication recommendation capabilities, particularly in scenarios involving patients with infrequently occurring health conditions.
These findings underscore the superiority of RAREMed in providing precise medication recommendations for patients with rare diseases, thereby showcasing its potential in addressing the fairness concern within the realm of medication 
recommendation.

\begin{figure}[h]
\centering
\includegraphics[width=0.475\textwidth]{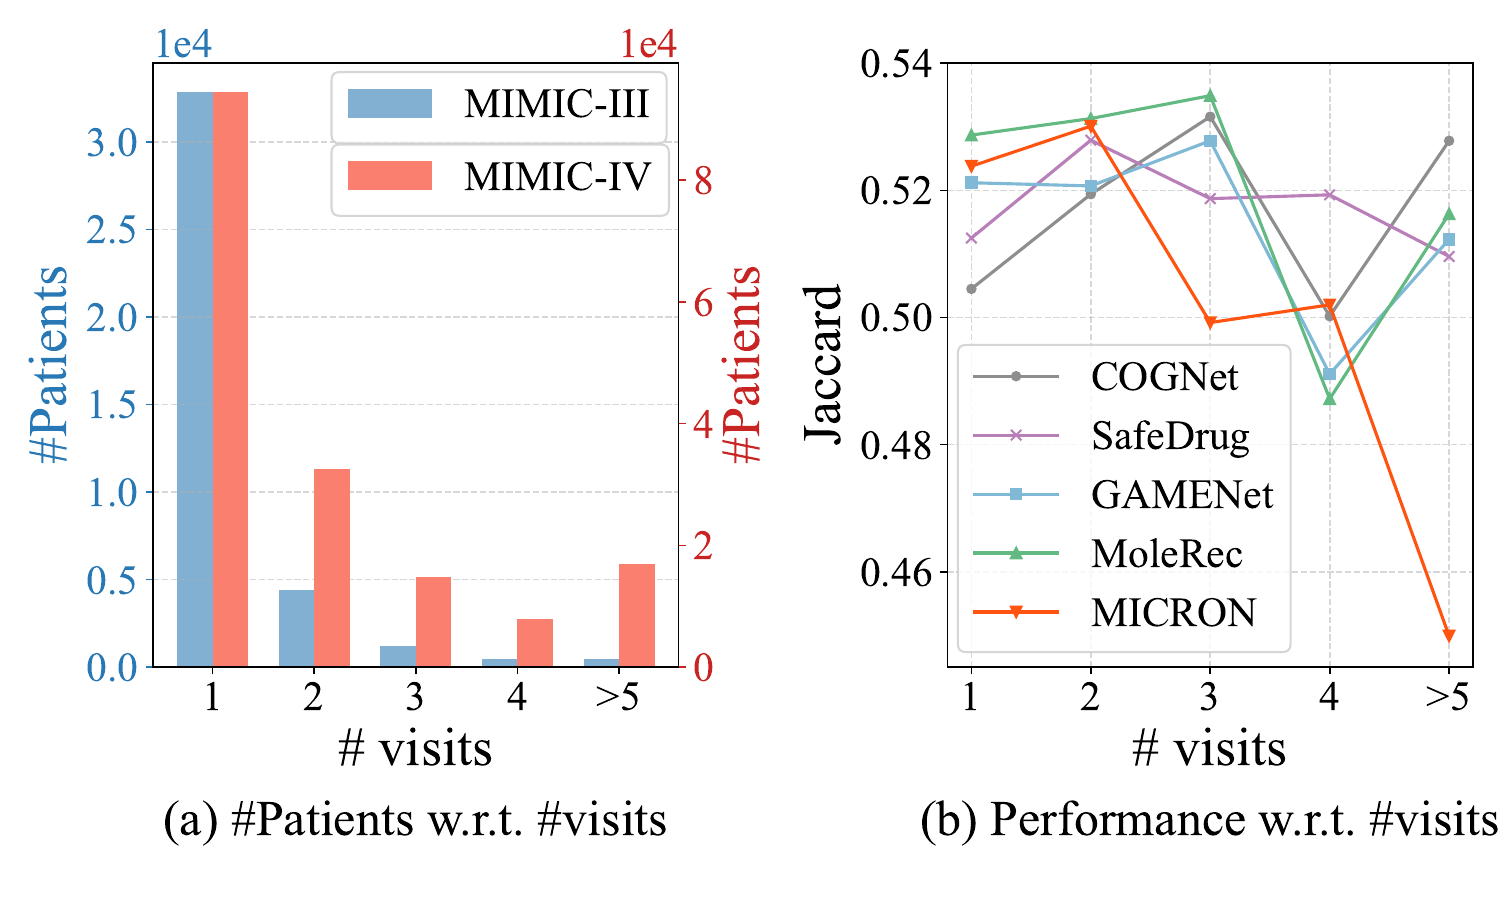}
\caption{(a) Skewed distribution of \#visits in EHR.
% We tally the patient count across various visit numbers. 
(b) Medication accuracy across different visit numbers of several representative longitudinal-based methods on MIMIC-III.}
\label{fig:diff_visit}
\end{figure}

\subsection{Importance of Single-Visit Patients}
\label{appen: single}
In this section, we present the rationale behind our choice to develop RAREMed as an instance-based method, focusing on the effective utilization of clinical information from the current visit. We discuss this decision from two key perspectives:

\begin{itemize}[leftmargin=*]
    \item \textbf{Dominance of single-visit patients in EHR data:} Real EHR datasets exhibit a prominent trend, as depicted in Figure~\ref{fig:diff_visit} (a), wherein a significant majority of patients have only a single visit recorded. This observation accurately reflects the prevailing real-world scenario, where most patients are first-time visitors. Moreover, privacy considerations further hinder the comprehensive utilization of patients' historical information. Therefore, it is crucial to develop methods that can effectively leverage the clinical information available at the current visit to provide accurate and reliable recommendations for this majority population.
    
    \item \textbf{Challenges in leveraging historical information:} Existing approaches that rely on historical information often fail to deliver satisfactory results due to incomplete exploitation of such data. Notably, models such as GAMENet~\cite{gamenet}, SafeDrug~\cite{safedrug} and MoleRec~\cite{molerec} leverage RNN to encode historical information, 
    % resulting in limited overall accuracy advantages, as shown in Table~\ref{tab:single} and Table~\ref{tab:multi}. Furthermore, 
    while the accuracy does not exhibit significant growth as the number of visits increases, as shown in Figure~\ref{fig:diff_visit}(b). COGNet~\cite{cognet} introduces a copy-or-predict mechanism to copy medication information from similar historical visits. However, this approach can be easily replicated by doctors, thereby diminishing its value. MICRON~\cite{micron} focuses on medication changes between visits, but the     prediction errors tend to accumulate as the number of visits increases, evidenced by the decreasing trend in Figure~\ref{fig:diff_visit}(b). In summary, effectively leveraging historical information remains a challenging task, which we acknowledge as an important  area for future research.
\end{itemize}

In summary, our focus on single-visit patients in developing RAREMed is justified by the dominance of such patients in real-world EHR data and the challenges associated with effectively utilizing historical information. By prioritizing the clinical information available at the current visit, we aim to provide accurate and reliable medication recommendations that address the specific needs of this majority population.
